# Supplementary material for: Evaluating Graphical Perception with Multimodal LLMs
Source: arXiv:2504.04221 source file (2025-04-05)
Supplement: Supplementary file 1 [file Appendix.tex]

\textbf{Experiment 1}

Our prompts are:

\begin{itemize}
    \item \textbf{Position Common Scale}: Estimate the block's vertical position (range: 0-60, top to bottom). Number only. No explanation.
    \item \textbf{Position Non-Aligned Scale}: Estimate the block's vertical position (range: 0-60, top to bottom). Number only. No explanation.
    \item \textbf{Length}: Estimate the line length from top to bottom (range: 0-100). Number only. No explanation.
    \item \textbf{Direction}: Estimate the line's direction (range: 0-359 degrees). Number only. No explanation.
    \item \textbf{Angle}: Estimate the angle (range: 0-90 degrees). Number only. No explanation.
    \item \textbf{Area}: Estimate the area of a circle, ensuring your answer falls within the range of 3.14 to 5026.55 square units. Assume the circle fits within a 100x100 pixel image. Provide only the numeric value, no explanation.
    \item \textbf{Volume}: Estimate the volume of a cube, with your answer restricted to the range of 1 to 8000 cubic units. Assume the cube fits within a 100x100 pixel image. Provide only the numeric value, no explanation.
    \item \textbf{Curvature}: Estimate the line curvature (range: 0.000 to 0.088) of a Bezier curve constrained within a 100x100 pixel space. Provide only the numeric curvature value (up to 3 decimal places), no explanation.
    \item \textbf{Shading}: Estimate shading density (range: 0-100). Number only. No explanation.
\end{itemize}

\textbf{Experiment 2}

Both bar and pie chart has separated prompt as mentioned in Appendix, however they mostly have similar zero-shot prompting structure:

The pie or bar chart you are looking at is created as follows: 

\begin{itemize}
    \item First, create a list of five values where each value is between 3 and 39, and all values add up to 100. "
    \item Next, divide each value in the list by the largest value, so that the largest value becomes 1.0.
    \item Now, look at the pie chart again.
    \item Identify the largest segment, which is marked with a dot.
    \item Estimate the ratio of the other four values to maximum.
    \item Format your answer as [1.0, x.x, x.x, x.x, x.x].

\end{itemize}

The difference between two tasks prompts are how all models estimate the ratio of the other four values to maximum:
\begin{itemize}
    \item Pie chart: Go counterclockwise around the pie starting from the largest segment, estimating the ratio of the other four values to the maximum.
    \item Bar chart: Move left to right along the bar chart starting from the largest bar, estimating the ratio of the other four values to the maximum.
\end{itemize}

\section {Experiment 3}

Our zero-shot prompts for all five tasks are as follows:

Type 1, Type 2, and Type 3 have a similar prompt structure, with the only differences being the chart types: grouped, divided, and mixed bar charts. The prompt is: 

\textit{In the grouped/divided/mixed bar chart, compare the heights of the two marked bars. Estimate the ratio of the height of the shorter marked bar to the height of the taller marked bar. Use a scale from 0 to 1, where 1 indicates that both marked bars are of equal height. No explanation.}

Type 4 and Type 5 also have a similar prompt structure, with the distinction being between divided stacked bars and the left bar of the mixed divided stacked bar chart. The prompt is: 

\textit{In the divided stacked bars or the left bar of the mixed divided stacked bar chart, compare the lengths of the two marked segments in the left and right bars. Estimate the ratio of the shorter marked segment’s length to the length of the taller marked segment. Use a scale from 0 to 1, where 1 indicates equal length. No explanation.

\section {Experiment 4}

Our zero-shot prompting for these two tasks are: \textit{Estimate the lengths of the two bars without framing OR frame. Both lengths should fall between 49 and 60 pixels. No explanation. Format of the answer [xx, xx].}

\section {Experiment 5}

Our research also includes zero-shot prompts for this experiment to instruct our models to regress values for all three tasks. Our prompts are:

\begin{itemize}
    \item \textbf{Task 10}: Please estimate how many dots were added to the initial 10 dots. The answer must be within the range of 1 to 10. Number only. No explanation.
    \item \textbf{Task 100}: Please estimate how many dots were added to the initial 100 dots. The answer must be within the range of 1 to 10. Number only. No explanation.
    \item \textbf{Task 1000:} Please estimate how many dots were added to the initial 1000 dots. The answer must be within the range of 1 to 10. Number only. No explanation.
    \item 
\end{itemize}
